# Supplementary material for: Multi-view Tracking Using Weakly Supervised Human Motion Prediction
Source: arXiv:2210.10771 source file (2022-10-19)
Supplement: Supplementary file 1 [file supp.tex]

\section{Varying the number of viewpoints}
We propose to evaluate the impact of using multiple viewpoints on detection accuracy. We train multiple models and vary the number of views they are given.
Results can be found in \cref{fig:supp_views}, it shows a steady increase in MODA when the number of views is increased.
Note that the largest jump in performance occurs when switching from one to two views. By having opposing views, the model can easily resolve error due to occlusions.
% !TEX root = ../top.tex
% !TEX spellcheck = en-US

\begin{figure}[h]
    \begin{center}
    %   \centering\includegraphics[width=0.80\textwidth]{./figs/archi_global_3.png}
    \centering\includegraphics[width=1\linewidth]{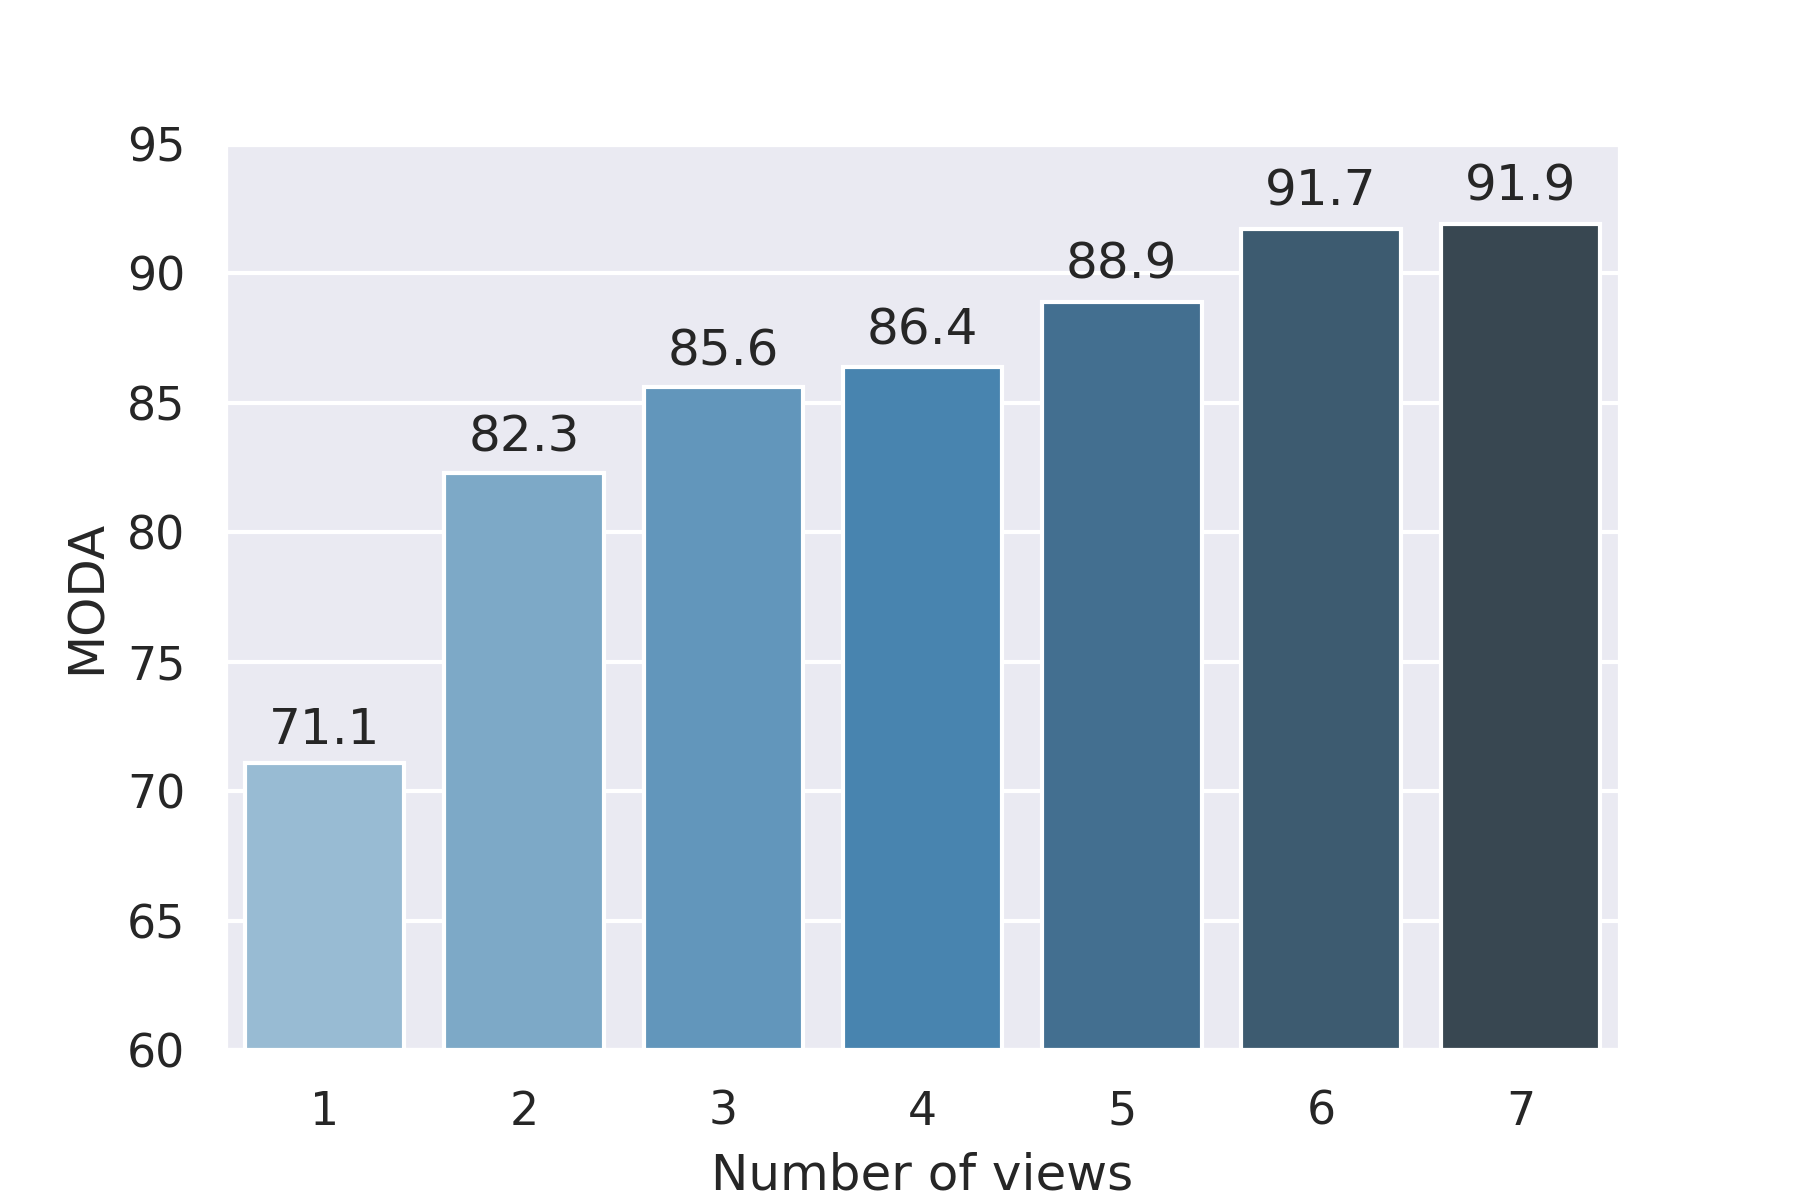}
    \end{center}
    % need to be reworded copy from 2018 paper
    \caption{\textbf{Effect of the number of views on MODA}. We use the WILDTRACK dataset to evaluate the effect of having multiple view on the detection accuracy measured using MODA.
    The accuracy increase steadily with the number of view until it reaches a plateau around 6 views.
    }
    \label{fig:supp_views}
    \end{figure}

 \section{Comparison to Appearance based tracking}
 
\begin{table*}[h]
    \begin{center}
    \begin{tabular}{r  c c c c c c c } \toprule
    &  \multicolumn{6}{c}{WILDTRACK dataset}  \\ \cmidrule(lr{.75em}){2-7}
    model & MOTA & MOTP & IDF1 & IDP & IDR & ML & MT   \\ \midrule
    MvMHAT \cite{gan2021self} & -3.29 & 1.31 & 19.9 & 12.2 & 54.6 & 14 & 13 \\
    MvMHAT \cite{gan2021self} (Single View) & 36.1 & 1.15 & 52.3 & 66.8 & 43.0 & 23 & 12 \\
    MVFlow + muSSP Single View (Ours) & \textbf{69.5} & \textbf{0.62} & \textbf{63.9} & \textbf{69.3} & \textbf{59.3} & \textbf{1} & \textbf{18} \\
    \bottomrule
    \end{tabular}
    \end{center}
      \caption{\textbf{Multi-view multi-person tracking} We evaluate an appearance-based model, which doesn’t rely  on any assumptions about scene structure, camera position of human motion.
      It uses pre-extracted bounding box, and reconstruct track by matching bounding box across time and viewpoints. We use WILDTRRACK ground truth bounding boxes both for training and evaluation.
      When using multiple views, the model fail to match people across viewpoints resulting in a large number of false positive and low tracking performances.
      Using a single view improve the tracking performance. Still, our proposed approach by leveraging camera calibration and  prediction human motion obtains higher MOTA even in the single view use case.
      }  
     \label{tab:mvmtracking_supp}
\end{table*}

    %Xu, Yuanlu, et al. "Cross-view people tracking by scene-centered spatio-temporal parsing." Proceedings of the AAAI Conference on Artificial Intelligence. Vol. 31. No. 1. 2017.

Apperance based tracking methods have gained a lot of traction in the past few years. In particular the human re-identification task.
As opposed to our approach these methods, make no assumption about the scene or human motion and entirely rely on the appearance of the person they are trying to track. For the sake of completeness, we compare our approach to one of those methods. We train and evaluate MvMHAT \cite{gan2021self} on the WILDTRACK dataset and report the results in \cref{tab:mvmtracking_supp}. Since MvMHAT relies on pre-extracted detections, we use ground truth detections both for training and evaluation. The resulting tracks are then projected in the ground plane for evaluation. Projections from different views with the same person ID are merged together. MvMHAT results are provided in the first line of \cref{tab:mvmtracking_supp}.
 With a negative MOTA due to a large number of false positive, MvMHAT fail to associate detections coming from different views. We suspect it is due to the small size of WILDTRACK.
 To discard false positive due to missed view association we also report evaluation on the single best view (second line of \cref{tab:mvmtracking_supp}). With a MOTA of 36.1, MvMHAT is outperformed by our model (train on a single view)  with a large margin. While this comparison is not fair, this experiment highlights the benefits of dedicated methods leveraging strong assumption about human motion and view alignment (calibration).

\section{Qualitative results}
 We provide additional qualitative results in \cref{fig:visu_flow_supp}. The supplementary archive contains a video showing our results on both WILDTRACK and PETS. It illustrates the reduction in identity switch when using the human flow predicted by our model.

 % !TEX root = ../top.tex
% !TEX spellcheck = en-US

\begin{figure*}[h]

        \centering
        \begin{subfigure}[b]{0.235\textwidth}  
            \centering 
            \includegraphics[width=\linewidth]{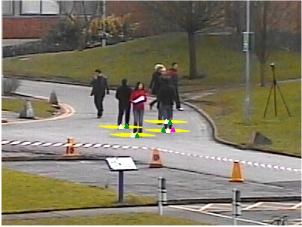}
        \end{subfigure}
        \hfill
        \begin{subfigure}[b]{0.235\textwidth}
            \centering
            \includegraphics[width=\linewidth]{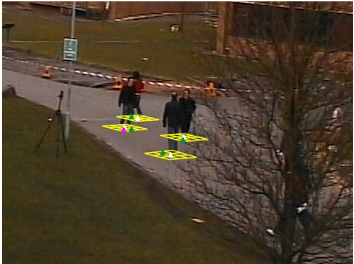}
        \end{subfigure}
        \hfill
        \begin{subfigure}[b]{0.235\textwidth}
            \centering
            \includegraphics[width=\linewidth]{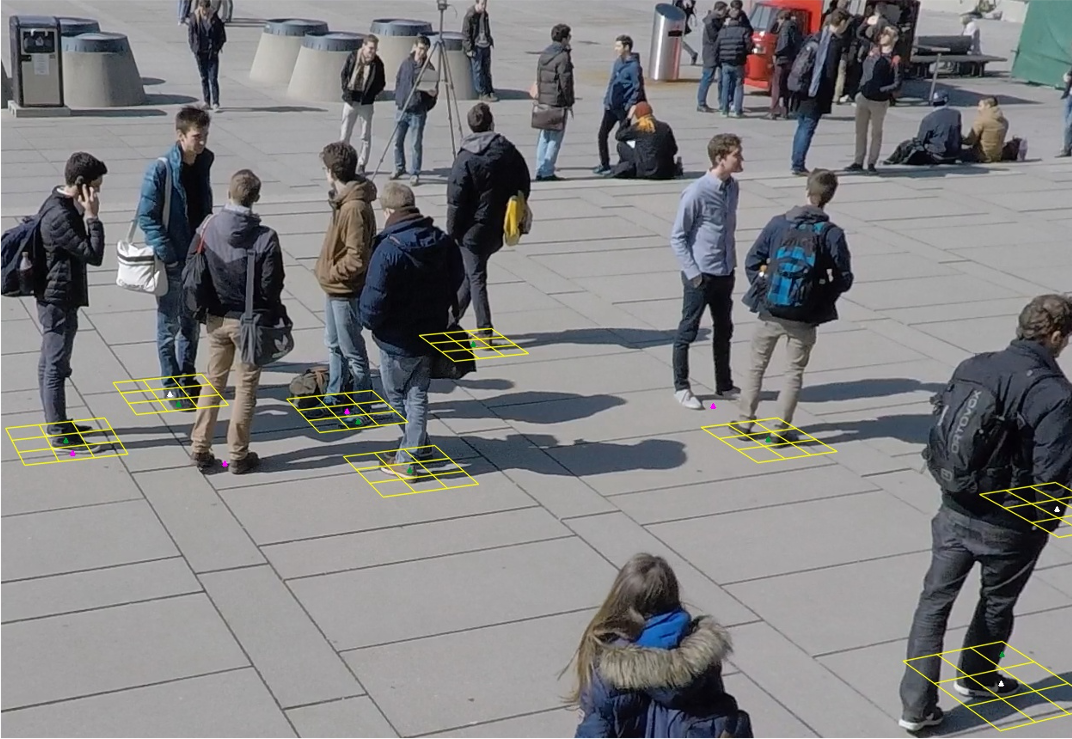}
        \end{subfigure}
        \hfill
        \begin{subfigure}[b]{0.235\textwidth}  
            \centering 
            \includegraphics[width=\linewidth]{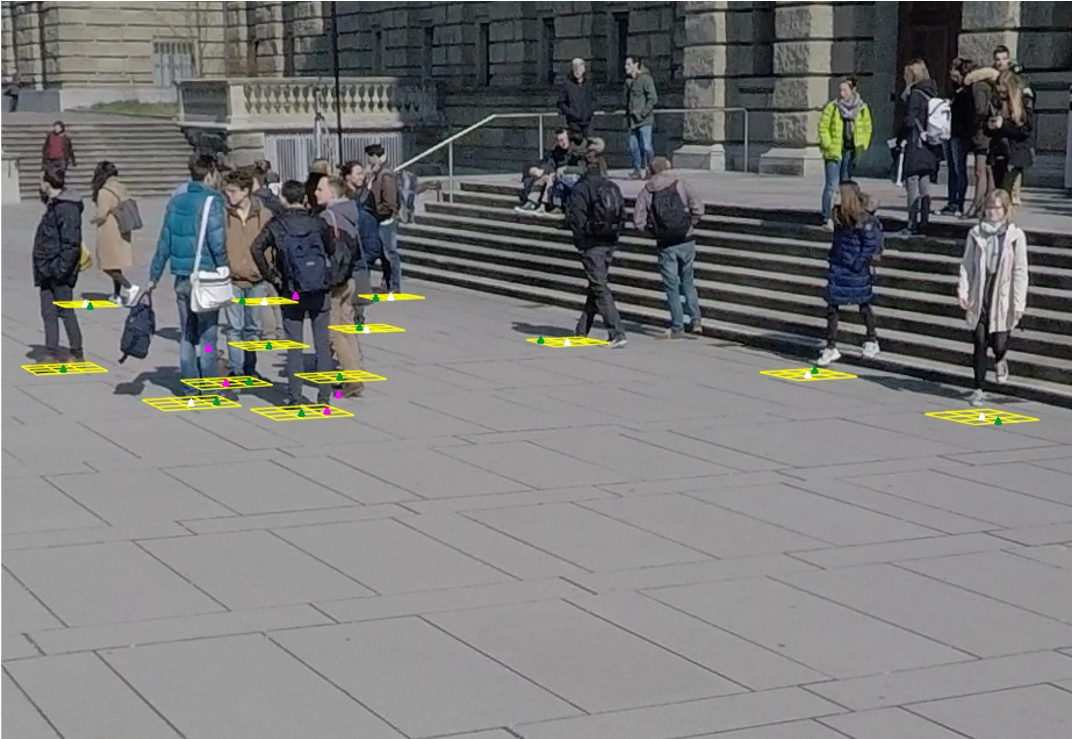}
        \end{subfigure}

    \caption{\textbf{Visualization of the predicted flow, viewed best zoomed in.}. For each detected person in the image, we visualize the predicted flow.
    Centered around each detection we reproject a $3 \times 3$ grid corresponding to the ground plane division.
    The green triangle mark the cell of the flow direction with the highest probability. Or, in other words, the predicted position for the next time step.
    If the prediction is incorrect, a pink dot marks the true destination. Note that ground truth flow is used for visualization purpose only and is never used during training.
    The two images on the left are coming from the PETS2009 dataset, the two on the right one are coming from the WILDTRACK dataset.
    }
    \label{fig:visu_flow_supp}
    \end{figure*}

\section{Failure mode analysis}
The proposed method makes multiple assumptions about human motion and scene configuration. In this section we propose to use the WILDTRACK dataset to evaluate how our model behave in case those assumptions are broken.

\subsection{Breaking motion distance constraints}
Assuming the proposed model is trained on data which mostly follow assumptions defined in Section 3.2, we evaluate how our model performs on inputs that violate the people conservation constraint defined in Eq 1. We artificially violate this constraint by sampling frames that are far apart such that the motion of the people in between the two frames is greater than one ground plane grid cell.

If the motion length is bigger than one, it is not possible for the model to predict flow that respect both constraint defined in Eq 1 and Eq 3. It means that the predicted flows will be incorrect. However we observed in \cref{fig:abla_run_supp}, that the reconstructed detection maps are mostly correct. In particular we observe two failure modes, if the motion length is longer than one grid cell but smaller than  four cells the model reconstruct a single detection (circled in green). The second failure mode is observed when the motion is longer than three cells, in that case the model reconstruct two detections one for the starting point and one for the ending point of the motion (circled in red). Tracker algorithms such as muSSP or KSP can handle such noises. Occasional violation of the motion assumption would have minimal effect on the overall tracking performance.

Note that in the current configuration a grid cell is 20 cm. To consistently violate the motion constraint with 5 fps videos a person should move more than 30 cm between each frame which correspond to a speed of 5.4 km/h. In the example above, we've seen that for motion up to 3 cells the detection are mostly correct. Moving more than 3 cells between two frames would require a speed higher than 16.2 km/h which would be very uncommon in everyday scenarios. Moreover handling such high-speed scenarios would only require to capture data at higher framerate.

 % !TEX root = ../top.tex
% !TEX spellcheck = en-US

\begin{figure*}[h]
            \centering 
            \includegraphics[width=\linewidth]{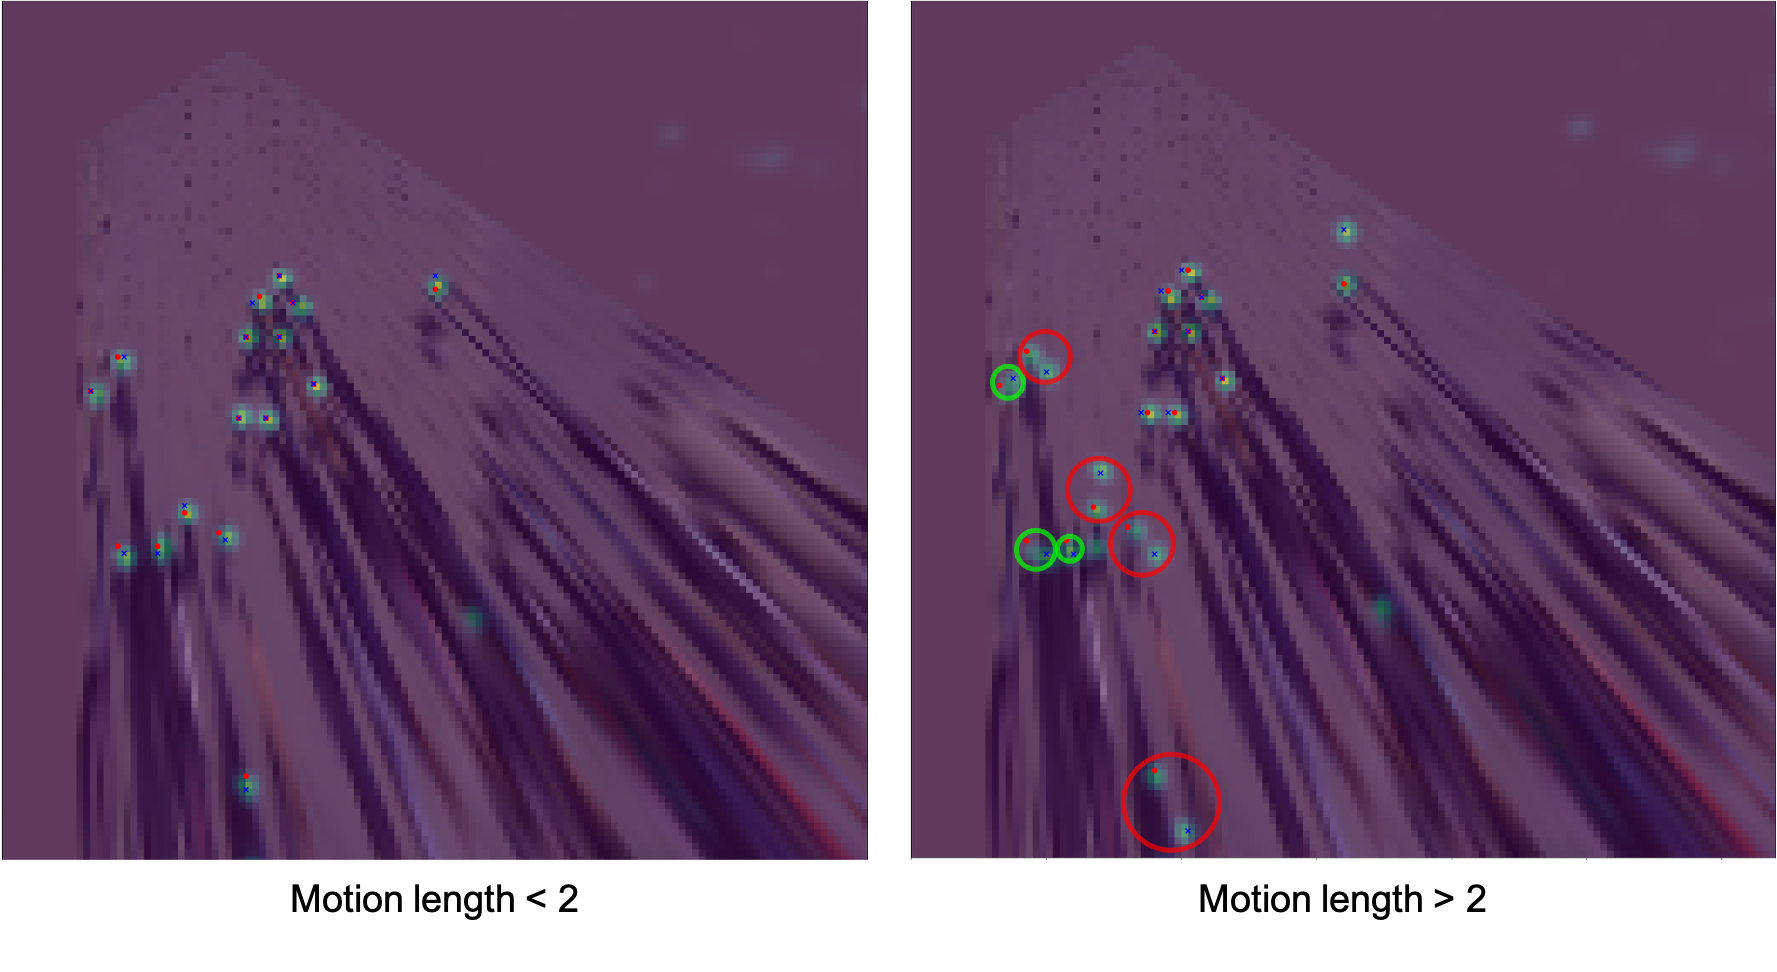}

    \caption{\textbf{Failure analysis, breaking the maximum motion length constraint.} We evaluate the robustness of the proposed model when operating outside of its motion length assumption.
    The detection heatmap is overlaid on top of the ground plane projection of the scene, the red dot corresponds to the ground truth detections at time $t$ and the blue crosses to the ground truth detections in the next time step $t+n$.
    The left image corresponds to detection obtain in a normal setting where $n=1$, the right image is obtained with $n=10$ resulting in motion length of 8, 5, 4, 3, 3, 2 cells violating the model assumption.
    Two failure modes are observed: Detections circled in green where the flow is incorrect but the detection reconstruction is still valid.  Detections circled in red, the flow is incorrect and the model reconstruct two detections one for the start of the motion and one for the end.
    }
    \label{fig:abla_run_supp}
    \end{figure*}

\subsection{Introducing error in the calibration}
To evaluate the robustness of our model to calibration error, we modify the extrinsic parameters of camera 2 and add 50 cm to its Z coordinate. This change will result in incorrect ground plane projection for the frames coming from that camera, by projecting the frame to a plane 50 cm above the ground plane and therefore shifting spatially every person.

We test our model in two scenarios and report the results in \cref{tab:failure_analysis}. First we direclty evaluate our best model which was trained with the correct calibration. While performances are degraded, the model doesn't collapse completely and results remain reasonable. Note that muSSPFlow which use the predicted motion is more robust than the original muSSP and achieve a higher MOTA.
For the second scenario, we retrain a model from scratch using the corrupted calibration. The performance after retraining are improved by almost 6 points, showing the benefit of our end-to-end trainable model which can learn to compensate for large calibration error.

\section{Ground plane discretization ablation}
We propose to evaluate the impact of the discretization of the ground  plane on the overall tracking performance.
In the model a single cell on the ground plane correspond to a 20x20cm square in the real word. We train two new models where the cells have been scaled by a factor of 0.8 and 1.2. When the grid cells are scaled down by a factor of 0.8 it introduces peoples moving more than one grid cell (0.74\% of movement are longer than 1), and when they are scaled up by a factor of 1.2 it introduces overlapping peoples (4 peoples over the dataset instead of 0). In both cases the tracking performance suffers, results can be found in \cref{tab:discretization_abla}. In practice there is a range of optimal values for the grid size that can be derived from the data, and directly depends on the density and speed of people in the scene and the framerate of the videos.

\begin{table*}[h]
    \begin{center}
    \begin{tabular}{r  c c c c c c c } \toprule
    &  \multicolumn{6}{c}{WILDTRACK dataset}  \\ \cmidrule(lr{.75em}){2-7}
    model & MOTA & MOTP & IDF1 & IDP & IDR & ML & MT   \\ \midrule
    MVFlow + muSSP + calib error & 80.9 & 0.56 & 78.2 & 79.3 & 77.1 & 3 & 29 \\
    MVFlow + muSSPFlow + calib error & 81.1 & 0.55 & 77.5 & 78.6 & 76.4 & 3 & 29 \\
    MVFlow + muSSP + calib error + retrained & 86.6 & 0.51 & 85.8 & 85.2 & 86.5 & 2 & 34 \\
    MVFlow + muSSPFlow + calib error + retrained & 87.0 & 0.51 & 86.0 & 85.4 & 86.7 & 2 & 34 \\

    \end{tabular}
    \end{center}
    
      \caption{\textbf{Failure Analysis: calibration errors} We evaluate the robustness of our model to error in camera calibration. 
      Using the WILDTRACK dataset we introduce an error by moving a single camera 50cm on it's z axis. We provide results for our model trained with correct calibration and one retrained with the erroneous calibration.
      }  
     \label{tab:failure_analysis}
\end{table*}

    %Xu, Yuanlu, et al. "Cross-view people tracking by scene-centered spatio-temporal parsing." Proceedings of the AAAI Conference on Artificial Intelligence. Vol. 31. No. 1. 2017.

\begin{table*}[h]
    \begin{center}
    \begin{tabular}{r  c c c c c c c } \toprule
    &  \multicolumn{6}{c}{WILDTRACK dataset}  \\ \cmidrule(lr{.75em}){2-7}
    model & MOTA & MOTP & IDF1 & IDP & IDR & ML & MT   \\ \midrule
    MVFlow + muSSP + 0.8 grid scale & 87.0 & 0.66 & 92.2 & 91.7 & 92.71 & 2 & 36 \\
    MVFlow + muSSP + 1.2 grid scale & 90.6 & 0.44 & 86.6 & 84.7 & 87.9 & 2 & 39 \\
    % MVFlow + muSSP  & 91.3 & 0.57 & 93.5 & 92.7 & 94.2 & 2 & 38 \\
    \end{tabular}
    \end{center}
    
      \caption{\textbf{Ground plane discretization ablation} We evaluate the impact of the ground plane grid size over the tracking performance on the WILDTRACK dataset. We train and evaluate two new models where the grid cells have been scaled by a factor of 0.8 and 1.2. In both cases the performances drop compared to the original model.
      }  
     \label{tab:discretization_abla}
\end{table*}

    %Xu, Yuanlu, et al. "Cross-view people tracking by scene-centered spatio-temporal parsing." Proceedings of the AAAI Conference on Artificial Intelligence. Vol. 31. No. 1. 2017.

\section{Implementation details}
The method is implemented in pytorch and trained on a single Nvidia v100.

\paragraph{Feature extraction} The feature extraction module consists of a Resnet 54 pretrained on imagenet classification. The last four layers are removed and the features extracted are of dimensionality 128. 

\paragraph{Ground plane projection}
The ground plane projection is based on the \textit{grid\_sample} pytorch function which implements \cite{Jaderberg15}. The homography $H$ corresponding to the ground plane projection is obtained as follows:
$$ H = KR_T, $$
where $K$ are the intrinsic camera parameters and $R_T$ are the extrinsic camera parameters.

\paragraph{Temporal aggregation} Temporal aggregation consists of a concatenation of the features coming from the two timesteps applied on the channel dimension followed by a convolutional layer which brings back the number of channels to 128 and uses a 1x1 kernel.

\paragraph{Spatial aggregation}
The spatial aggregation module start by a convolutional layer with a kernel size of 5x5, it has $V$x128 channel input where $V$ is the number of views and 256 channel output.
It is followed by a batchnorm and a ReLU layer. A multiscale module which operates at 4 scales output the final human flow.
Each scale of the multiscale module consists of an Adaptive Average Pooling, followed by a 3x3 convolution, a batchnorm and a ReLU.
The output of all the scales are bilinearly interpolated to their original size, concatenated and the output goes through a final 1x1 convolution reducing their dimensionality to 9 followed by a sigmoid function to produce the human flow.

\section{Code}
The code of the model and training is provided in the following repository: \url{https://github.com/cvlab-epfl/MVFlow}

\section{Societal impact discussion}
Tracking is currently being used as a part of many useful applications for human robot interaction, autonomous driving, security, etc. However it can also be used negatively, such as for surveillance with little regard for people's privacy. This specific work aims to improve tracking accuracy and we hope that it is used responsibly. As with all open source research, it is the responsibility of the user to develop ethical products.
