# Supplementary material for: Multi-view Tracking Using Weakly Supervised Human Motion Prediction
Source: arXiv:2210.10771 source file (2022-10-19)
Supplement: Supplementary file 2 [file abla_run_supp.tex]

% !TEX root = ../top.tex
% !TEX spellcheck = en-US

\begin{figure*}[h]
            \centering 
            \includegraphics[width=\linewidth]{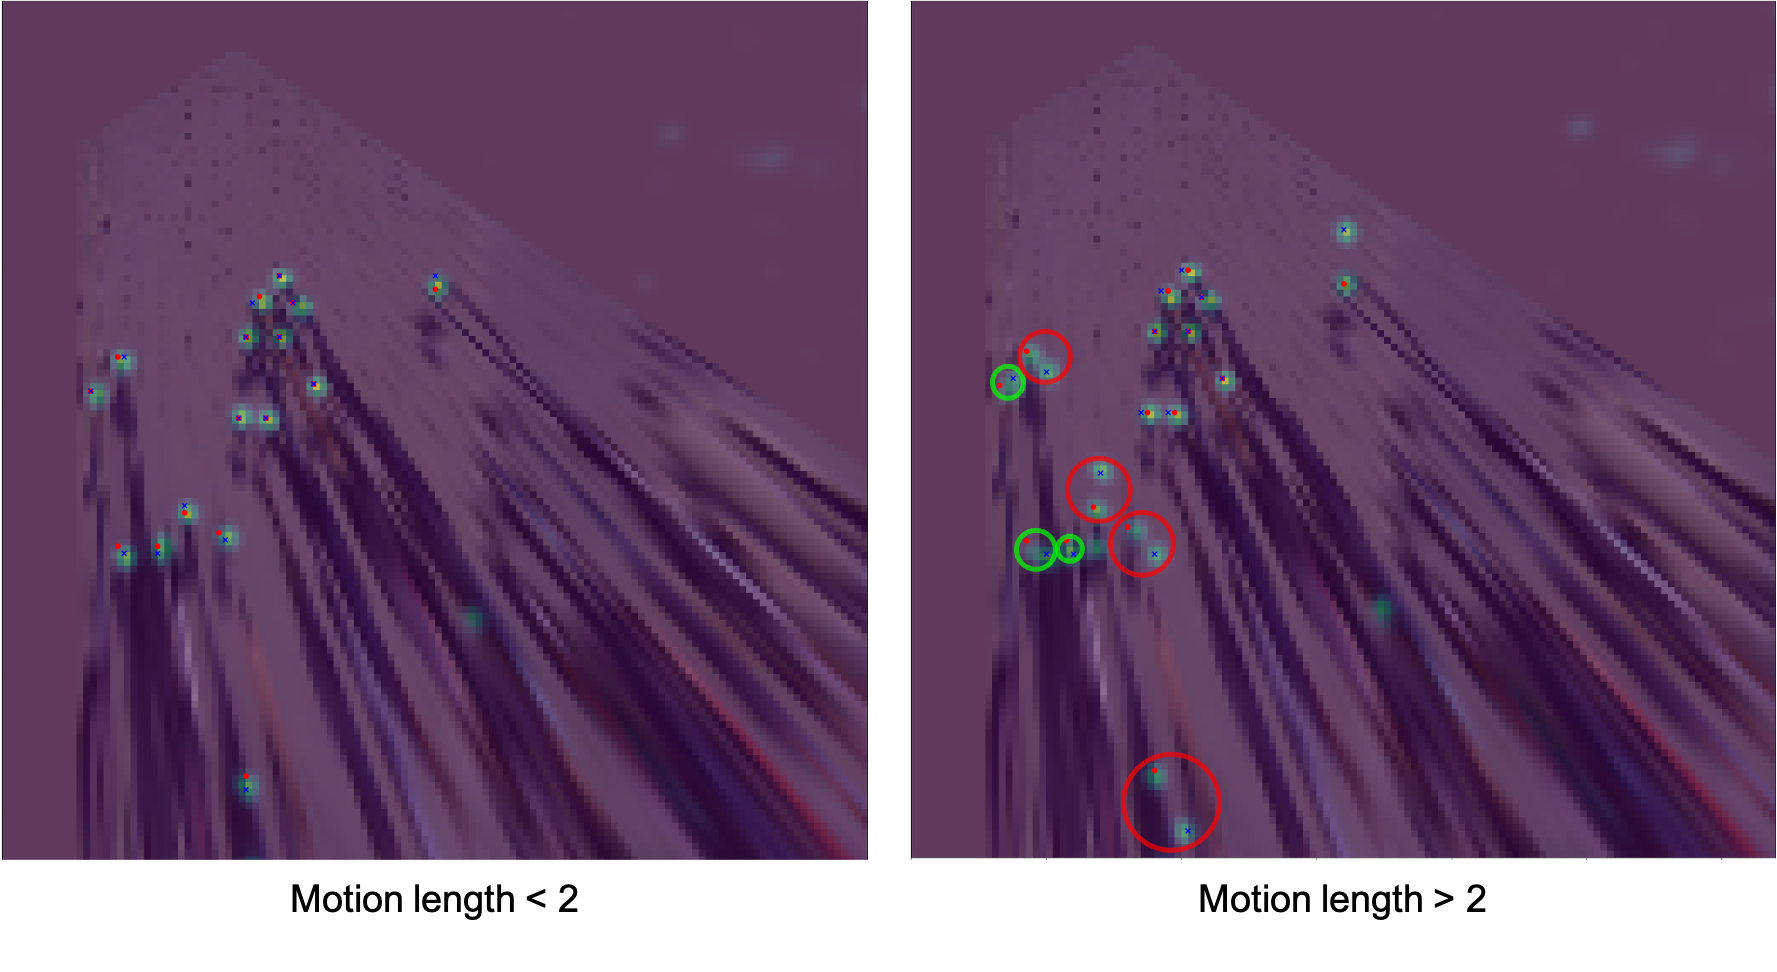}

    \caption{\textbf{Failure analysis, breaking the maximum motion length constraint.} We evaluate the robustness of the proposed model when operating outside of its motion length assumption.
    The detection heatmap is overlaid on top of the ground plane projection of the scene, the red dot corresponds to the ground truth detections at time $t$ and the blue crosses to the ground truth detections in the next time step $t+n$.
    The left image corresponds to detection obtain in a normal setting where $n=1$, the right image is obtained with $n=10$ resulting in motion length of 8, 5, 4, 3, 3, 2 cells violating the model assumption.
    Two failure modes are observed: Detections circled in green where the flow is incorrect but the detection reconstruction is still valid.  Detections circled in red, the flow is incorrect and the model reconstruct two detections one for the start of the motion and one for the end.
    }
    \label{fig:abla_run_supp}
    \end{figure*}
