# Supplementary material for: Multi-view Tracking Using Weakly Supervised Human Motion Prediction
Source: arXiv:2210.10771 source file (2022-10-19)
Supplement: Supplementary file 3 [file flow_results_supp.tex]

% !TEX root = ../top.tex
% !TEX spellcheck = en-US

\begin{figure*}[h]

        \centering
        \begin{subfigure}[b]{0.235\textwidth}  
            \centering 
            \includegraphics[width=\linewidth]{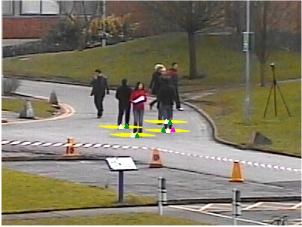}
        \end{subfigure}
        \hfill
        \begin{subfigure}[b]{0.235\textwidth}
            \centering
            \includegraphics[width=\linewidth]{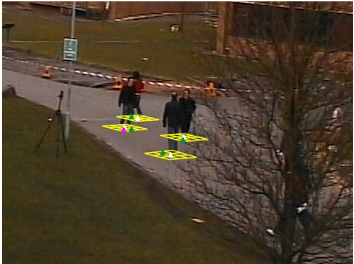}
        \end{subfigure}
        \hfill
        \begin{subfigure}[b]{0.235\textwidth}
            \centering
            \includegraphics[width=\linewidth]{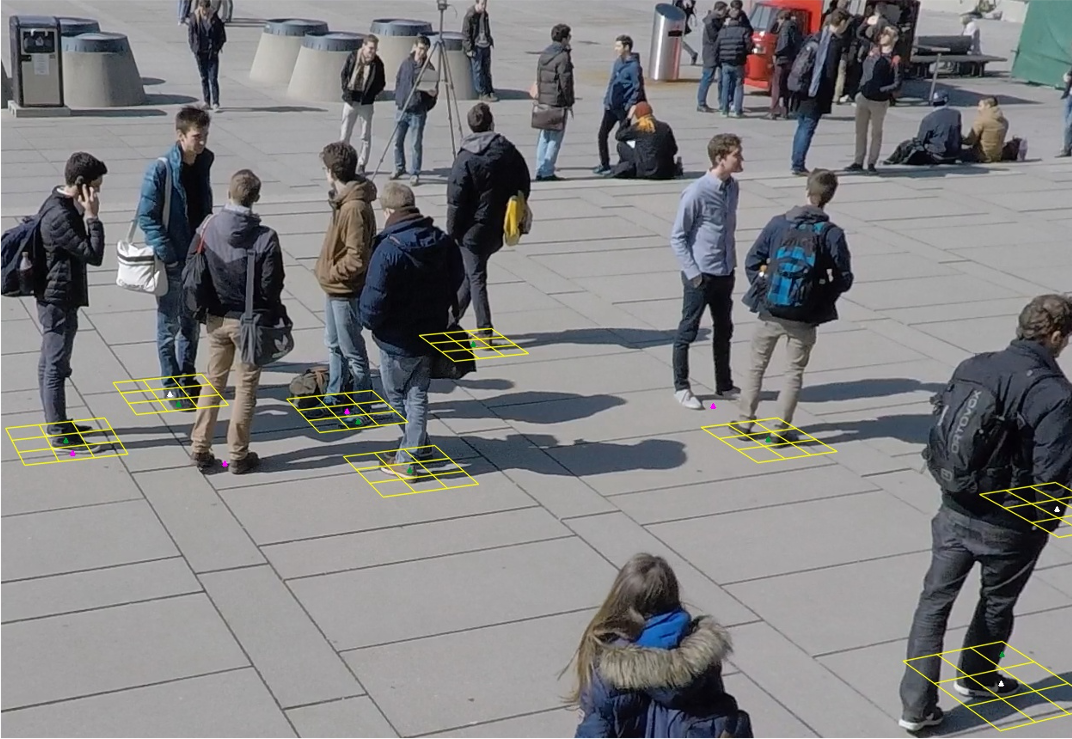}
        \end{subfigure}
        \hfill
        \begin{subfigure}[b]{0.235\textwidth}  
            \centering 
            \includegraphics[width=\linewidth]{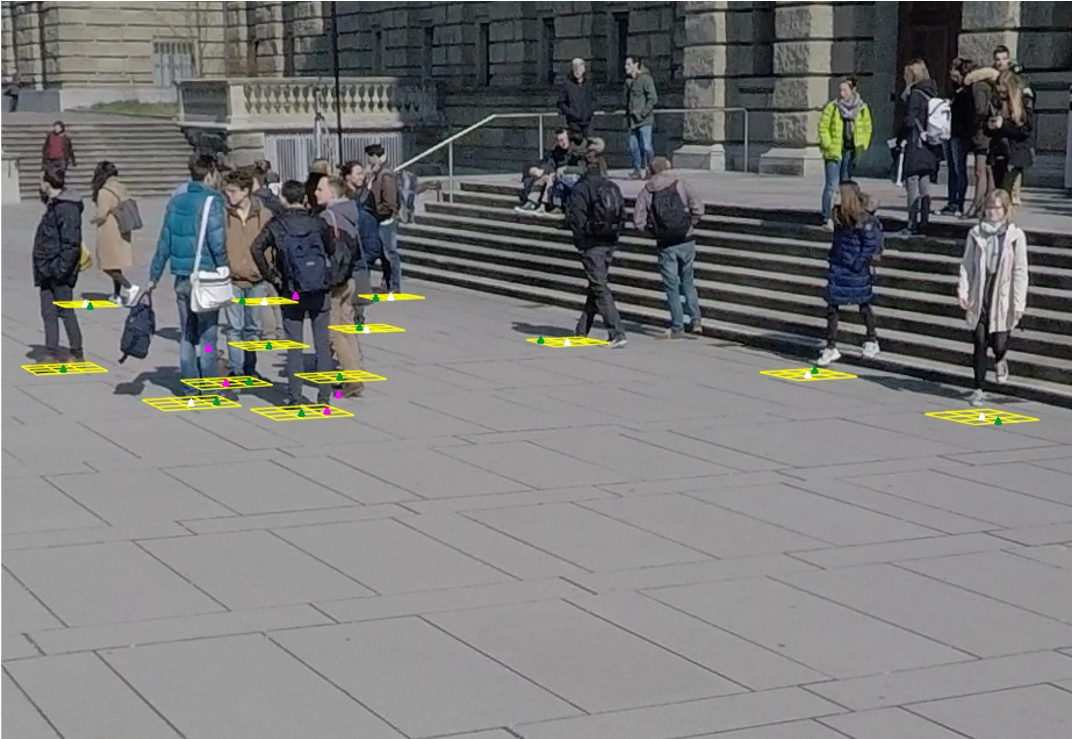}
        \end{subfigure}

    \caption{\textbf{Visualization of the predicted flow, viewed best zoomed in.}. For each detected person in the image, we visualize the predicted flow.
    Centered around each detection we reproject a $3 \times 3$ grid corresponding to the ground plane division.
    The green triangle mark the cell of the flow direction with the highest probability. Or, in other words, the predicted position for the next time step.
    If the prediction is incorrect, a pink dot marks the true destination. Note that ground truth flow is used for visualization purpose only and is never used during training.
    The two images on the left are coming from the PETS2009 dataset, the two on the right one are coming from the WILDTRACK dataset.
    }
    \label{fig:visu_flow_supp}
    \end{figure*}
