# Supplementary material for: Multi-view Tracking Using Weakly Supervised Human Motion Prediction
Source: arXiv:2210.10771 source file (2022-10-19)
Supplement: Supplementary file 4 [file supp_nb_views.tex]

% !TEX root = ../top.tex
% !TEX spellcheck = en-US

\begin{figure}[h]
    \begin{center}
    %   \centering\includegraphics[width=0.80\textwidth]{./figs/archi_global_3.png}
    \centering\includegraphics[width=1\linewidth]{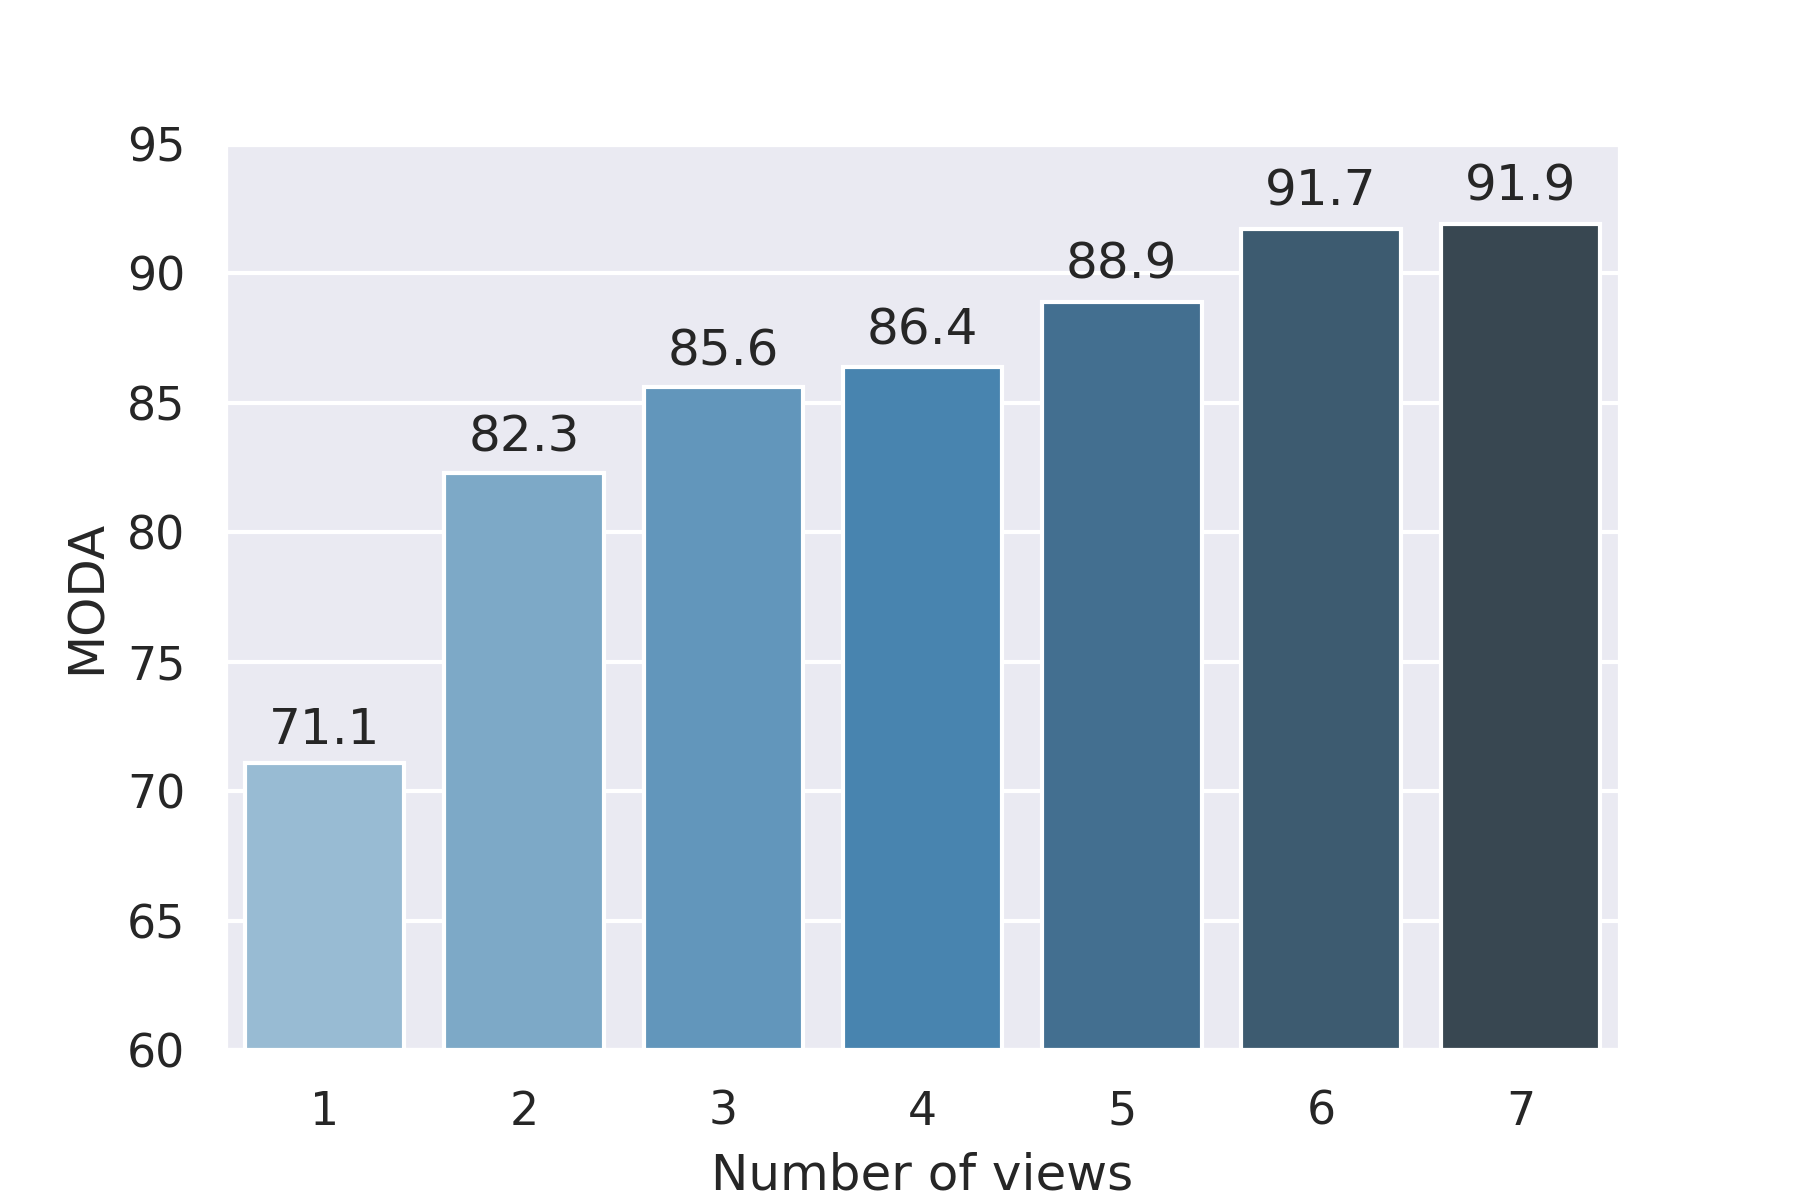}
    \end{center}
    % need to be reworded copy from 2018 paper
    \caption{\textbf{Effect of the number of views on MODA}. We use the WILDTRACK dataset to evaluate the effect of having multiple view on the detection accuracy measured using MODA.
    The accuracy increase steadily with the number of view until it reaches a plateau around 6 views.
    }
    \label{fig:supp_views}
    \end{figure}
