# Supplementary material for: Multi-view Tracking Using Weakly Supervised Human Motion Prediction
Source: arXiv:2210.10771 source file (2022-10-19)
Supplement: Supplementary file 5 [file discretization_abla_supp.tex]

\begin{table*}[h]
    \begin{center}
    \begin{tabular}{r  c c c c c c c } \toprule
    &  \multicolumn{6}{c}{WILDTRACK dataset}  \\ \cmidrule(lr{.75em}){2-7}
    model & MOTA & MOTP & IDF1 & IDP & IDR & ML & MT   \\ \midrule
    MVFlow + muSSP + 0.8 grid scale & 87.0 & 0.66 & 92.2 & 91.7 & 92.71 & 2 & 36 \\
    MVFlow + muSSP + 1.2 grid scale & 90.6 & 0.44 & 86.6 & 84.7 & 87.9 & 2 & 39 \\
    % MVFlow + muSSP  & 91.3 & 0.57 & 93.5 & 92.7 & 94.2 & 2 & 38 \\
    \end{tabular}
    \end{center}
    
      \caption{\textbf{Ground plane discretization ablation} We evaluate the impact of the ground plane grid size over the tracking performance on the WILDTRACK dataset. We train and evaluate two new models where the grid cells have been scaled by a factor of 0.8 and 1.2. In both cases the performances drop compared to the original model.
      }  
     \label{tab:discretization_abla}
\end{table*}

    %Xu, Yuanlu, et al. "Cross-view people tracking by scene-centered spatio-temporal parsing." Proceedings of the AAAI Conference on Artificial Intelligence. Vol. 31. No. 1. 2017.
