# Supplementary material for: Multi-view Tracking Using Weakly Supervised Human Motion Prediction
Source: arXiv:2210.10771 source file (2022-10-19)
Supplement: Supplementary file 6 [file failure_analysis_supp.tex]

\begin{table*}[h]
    \begin{center}
    \begin{tabular}{r  c c c c c c c } \toprule
    &  \multicolumn{6}{c}{WILDTRACK dataset}  \\ \cmidrule(lr{.75em}){2-7}
    model & MOTA & MOTP & IDF1 & IDP & IDR & ML & MT   \\ \midrule
    MVFlow + muSSP + calib error & 80.9 & 0.56 & 78.2 & 79.3 & 77.1 & 3 & 29 \\
    MVFlow + muSSPFlow + calib error & 81.1 & 0.55 & 77.5 & 78.6 & 76.4 & 3 & 29 \\
    MVFlow + muSSP + calib error + retrained & 86.6 & 0.51 & 85.8 & 85.2 & 86.5 & 2 & 34 \\
    MVFlow + muSSPFlow + calib error + retrained & 87.0 & 0.51 & 86.0 & 85.4 & 86.7 & 2 & 34 \\

    \end{tabular}
    \end{center}
    
      \caption{\textbf{Failure Analysis: calibration errors} We evaluate the robustness of our model to error in camera calibration. 
      Using the WILDTRACK dataset we introduce an error by moving a single camera 50cm on it's z axis. We provide results for our model trained with correct calibration and one retrained with the erroneous calibration.
      }  
     \label{tab:failure_analysis}
\end{table*}

    %Xu, Yuanlu, et al. "Cross-view people tracking by scene-centered spatio-temporal parsing." Proceedings of the AAAI Conference on Artificial Intelligence. Vol. 31. No. 1. 2017.
