# Supplementary material for: Multi-view Tracking Using Weakly Supervised Human Motion Prediction
Source: arXiv:2210.10771 source file (2022-10-19)
Supplement: Supplementary file 7 [file tracking_supp.tex]

\begin{table*}[h]
    \begin{center}
    \begin{tabular}{r  c c c c c c c } \toprule
    &  \multicolumn{6}{c}{WILDTRACK dataset}  \\ \cmidrule(lr{.75em}){2-7}
    model & MOTA & MOTP & IDF1 & IDP & IDR & ML & MT   \\ \midrule
    MvMHAT \cite{gan2021self} & -3.29 & 1.31 & 19.9 & 12.2 & 54.6 & 14 & 13 \\
    MvMHAT \cite{gan2021self} (Single View) & 36.1 & 1.15 & 52.3 & 66.8 & 43.0 & 23 & 12 \\
    MVFlow + muSSP Single View (Ours) & \textbf{69.5} & \textbf{0.62} & \textbf{63.9} & \textbf{69.3} & \textbf{59.3} & \textbf{1} & \textbf{18} \\
    \bottomrule
    \end{tabular}
    \end{center}
      \caption{\textbf{Multi-view multi-person tracking} We evaluate an appearance-based model, which doesn’t rely  on any assumptions about scene structure, camera position of human motion.
      It uses pre-extracted bounding box, and reconstruct track by matching bounding box across time and viewpoints. We use WILDTRRACK ground truth bounding boxes both for training and evaluation.
      When using multiple views, the model fail to match people across viewpoints resulting in a large number of false positive and low tracking performances.
      Using a single view improve the tracking performance. Still, our proposed approach by leveraging camera calibration and  prediction human motion obtains higher MOTA even in the single view use case.
      }  
     \label{tab:mvmtracking_supp}
\end{table*}

    %Xu, Yuanlu, et al. "Cross-view people tracking by scene-centered spatio-temporal parsing." Proceedings of the AAAI Conference on Artificial Intelligence. Vol. 31. No. 1. 2017.
